# Supplementary material for: Wettability of reentrant surfaces: a global energy approach
Source: arXiv:1710.11012 ancillary file (2017-10-31)
Supplement: Supplementary file 1 [file Supp_Info.pdf]

# Supporting Information for: "Wettability of reentrant surfaces: a global energy approach"

Marion Silvestrini and Carolina Brito*

*Instituto de Física, Universidade Federal do Rio Grande do Sul CP 15051, 91501-970 Porto Alegre, RS, Brazil*

E-mail: carolina.brito@ufrgs.br

In this supporting information (SI) we describe the algorithm used to find the thermodynamic wetting state for droplet placed on one of the three types of surfaces, the equations for the volume of the droplet in these three cases, the Potts Model employed in our simulations and show a table with simulation results for all the geometric parameters considered.

## Algorithm to find the thermodynamic wetting state

Fig.(S1) shows a flowchart of the algorithm to find the minimum energy for the both CB and W states, and then to decide which is the stable state of the system. The figure is build for the surface of type 1, but to expand this procedure for the surface of types 2 and 3, some modifications can easily be done. To apply it for the surface of type 2 [type 3], one has to set all parameters associated to this surface $(\mathrm{h}, \mathrm{a}, \mathrm{w}, \mathrm{h}_2, \mathrm{w}_2)$ [ $(\mathrm{h}, \mathrm{a}, \mathrm{w}, \mathrm{h}_2, \mathrm{w}_2, \mathrm{h}_3, \mathrm{w}_3)$ ] and the equation of energy for the W state to be minimized is Eq.(3) [ Eq.(4) ] instead of Eq.(2) and to compute the radius of the droplet it is necessary to solve the Eq.(S3) [ Eq.(S4) ] instead of Eq.(S2). We note that this algorithm allow us to know all the geometric parameters of the droplet (as the contact angle and its radius) in the stable state.

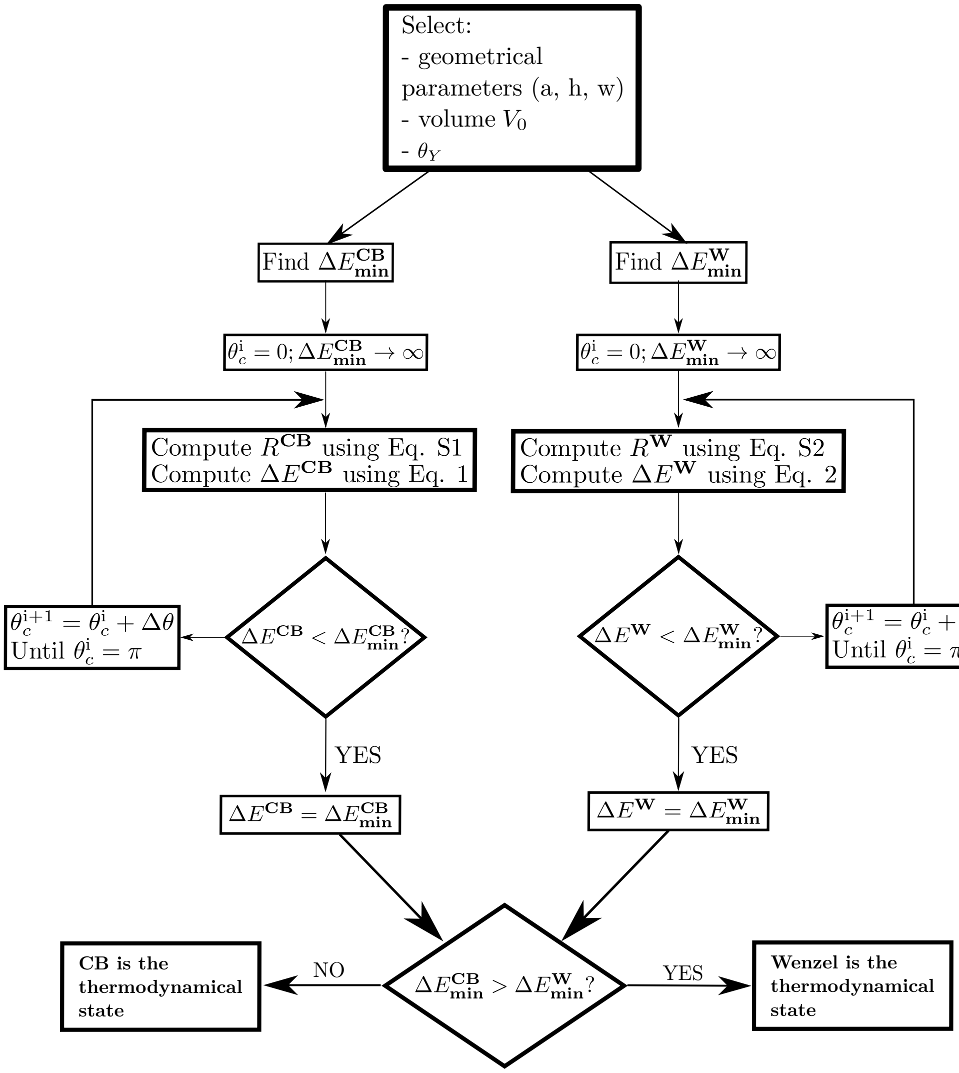


Figure S1: Schema of the algorithm to find the minimum state of droplet placed on surfaces of type 1. The generalization for surfaces of type 2 and 3 requires the modification of some equations and geometric parameters, as explained in the text.

## Equations for the volume of the droplet for the three types of surfaces

A volume of the cap of a sphere with radius $R$ and contact angle $\theta_C$ is given by:

$$V_{\mathrm{cap}}(R, \theta_C) = \frac{\pi}{12} R^3 \left(\cos(3\theta_C) - 9\cos(\theta_C) + 8\right). \tag{S1}$$

For the CB state the volume of the droplet is simply the volume of the spherical cap $V_{cap}(R^{\mathbf{CB}}, \theta^{\mathbf{CB}})$, while for the W state it is necessary to take into account the volume inside of the surface:

$$
\begin{aligned}
V^{\mathrm{W}}_{\mathbf{(1)}}(R^{\mathrm{W}}_{\mathbf{(1)}}, \theta^{\mathrm{W}}_{\mathbf{(1)}}) &= V_{\mathrm{cap}}(R^{\mathrm{W}}_{\mathbf{(1)}}, \theta^{\mathrm{W}}_{\mathbf{(1)}}) + \mathrm{N}^{\mathrm{W}}_{\mathbf{(1)}}(\mathrm{d}^2 - \mathrm{w}^2)\mathrm{h}, &\text{(S2)}\\
V^{\mathrm{W}}_{\mathbf{(2)}}(R^{\mathrm{W}}_{\mathbf{(2)}}, \theta^{\mathrm{W}}_{\mathbf{(2)}}) &= V_{\mathrm{cap}}(R^{\mathrm{W}}_{\mathbf{(2)}}, \theta^{\mathrm{W}}_{\mathbf{(2)}}) + \mathrm{N}^{\mathrm{W}}_{\mathbf{(2)}}\left[(\mathrm{d}^2 - \mathrm{w}^2)\mathrm{h} + (\mathrm{w}^2 - \mathrm{w}_2^2)\mathrm{h}_2\right], &\text{(S3)}\\
V^{\mathrm{W}}_{\mathbf{(3)}}(R^{\mathrm{W}}_{\mathbf{(3)}}, \theta^{\mathrm{W}}_{\mathbf{(3)}}) &= V_{\mathrm{cap}}(R^{\mathrm{W}}_{\mathbf{(3)}}, \theta^{\mathrm{W}}_{\mathbf{(3)}}) + \mathrm{N}^{\mathrm{W}}_{\mathbf{(3)}}\left[(\mathrm{d}^2 - \mathrm{w}^2)\mathrm{h} + (\mathrm{w}^2 - \mathrm{w}_2^2)\mathrm{h}_2 - 4\delta t(\mathrm{w} - t)\right]. &\text{(S4)}
\end{aligned}
$$

Because $N^{\mathrm{s}}_{\mathbf{(i)}} = \frac{\pi}{4}(2R^{\mathrm{s}}\sin(\theta^{\mathrm{s}}_{\mathrm{C}}/d)^2$, the equations of the volume are cubic in the variable $R$. Then, once the geometric parameters of the surface, $\theta_{\mathrm{Y}}$ and $\theta_{\mathrm{C}}$ are given, the solution for $R$ can be find analytically.

# Simulations of the Cellular Potts Model

In the reference[1] we have followed a previous 2D cellular Potts model (CPM)[2–4] and have extended it to the 3D counterpart to model the wetting behavior of a droplet of water on pillared surfaces. Here we recall the model and the parameters used in the simulation.

We model our system by a three state cellular Potts model on a simple cubic lattice. The Hamiltonian used is

$$H = \frac{1}{2}\sum_{<i,j>} E_{s_i,s_j}(1 - \delta_{s_i,s_j}) + \lambda(\sum_i \delta_{s_i,1} - V_T)^2 + mg\sum_i h_i\ \delta_{s_i,1}, \tag{S5}$$

where the spins $s_i \in \{0, 1, 2\}$ represent gas, liquid and solid states, respectively. The first summation ranges over pairs of neighbors which comprise the 3D Moore neighborhood in the simple cubic lattice (26 sites, excluding the central one); $E_{s_i,s_j}$ are the interaction energies of $s_i$ and $s_j$ of different states at interfaces and $\delta_{s_i,s_j}$ is the Kronecker delta. Changing the volume of the droplet has an energy cost: $V_T$ is the target droplet volume and $\lambda$ mimics its

compressibility; the second summation represents the total liquid volume, the total number of sites $i$ for which $s_i = 1$. The last term is the gravitational energy, with $g = 10\, m/s^2$. In both the volumetric and gravitational terms, only sites with liquid, $s_i = 1$, contribute.

To accept trial spin flips we use the standard Metropolis algorithm. Because only sites that are located at the droplet's frontier, i.e., at the liquid-gas or liquid-solid interfaces, do contribute to the change in energy, we optimize the code by keeping a list of these sites.[5] For the dynamics, one site at the interface, either liquid or gas, is chosen at random and a change in state between liquid and gas is accepted with probability $\min\{1, \exp(-\beta\Delta H)\}$, where $\beta = 1/T$ is the inverse of the effective temperature of the CPM.[6] $T$ acts as a noise to allow the phase space to be explored and the value $T = 13$ was used for all simulations. This value allows the system to fluctuate with an acceptance rate of approximately 22%. Each Monte Carlo step (MCS) is comprised of a number of trial spin flips equal to the total target volume of liquid, $V_T$.

The parameters for our Hamiltonian, Eq.(S5), were based on those used in experiments with water on a Polydimethylsiloxane (PDMS) surface[7] (surface tension of water $\sigma_{\text{GL}} = 70\, mN/m$ and $\sigma_{\text{SG}} = 25\, mN/m$, for the PDMS surface). In our numerical simulations, these values are divided by the number of neighboring sites that contribute to the first summation in Eq.(S5), that is, 26 neighboring sites. Our length scale is such that one lattice spacing corresponds to $1\, \mu m$. This implies that the interaction energies $E_{s_i,s_j} = \sigma_{ij} A$, with $A = 1\mu m^2$ being the unit area, are given by $E_{0,1} = 2.70 \times 10^{-9}\, \mu J$, $E_{0,2} = 0.96 \times 10^{-9}\, \mu J$ and $E_{1,2} = 1.93 \times 10^{-9}\, \mu J$. The third value is obtained from Young's relation $\sigma_{\text{GL}} \cos(\theta_{\text{Y}}) = \sigma_{\text{SG}} - \sigma_{\text{SL}}$, where $\theta = 111^\circ$ is the contact angle on a smooth surface. The mass existent in a unit cube is $m = 10^{-15} kg$. The value of $\lambda$ is chosen such that the fluctuations in volume around $V_T$ are smaller than energy changes due to interfacial trial spin flips. In simulations with $\lambda = 10^{-9} \mu J/(\mu m)^6$, fluctuations of less than 1% in volume are observed. Before applying the Potts model to simulate the droplet on a patterned surface, we verify its prediction for a flat surface. Using the parameters just specified, a contact angle of $\theta_C \approx 114^\circ$ is obtained in

our simulation, which is in good agreement with the experimental observation [7] of $(113 \pm 7)^\circ$ and very close to the value obtained from Young's relation, $\theta_{\mathrm{Y}} = 111^\circ$.

# Numerical values of $\theta_\mathrm{C}$

| a | h | TS | $\theta_1^{\mathrm{CB,sim}}(^\circ)$ | $\theta_1^{\mathrm{W,sim}}(^\circ)$ | $\mathrm{h}_2$ | TS | $\theta_2^{\mathrm{CB,sim}}(^\circ)$ | $\theta_2^{\mathrm{W,sim}}(^\circ)$ | $\mathrm{h}_3$ | TS | $\theta_3^{\mathrm{CB,sim}}(^\circ)$ | $\theta_3^{\mathrm{W,sim}}(^\circ)$ | $\mathrm{h}_3^*$ | Condition |
|---|---|---|---|---|---|---|---|---|---|---|---|---|---|---|
| 5 | 4 | W | $135.0 \pm 2.3$ | $124.7 \pm 0.0$ | | | | | | | | | | |
| | 6 | W | $138.9 \pm 0.0$ | $134.2 \pm 0.1$ | | | | | | | | | | |
| | 8 | CB | $138.4 \pm 1.0$ | $134.3 \pm 0.0$ | | | | | | | | | | |
| | 10 | CB | $138.8 \pm 0.1$ | $134.3 \pm 0.1$ | | | | | | | | | | |
| | 12 | CB | $138.4 \pm 1.0$ | $134.4 \pm 0.1$ | | | | | | | | | | |
| 6 | 4 | W | $135.0 \pm 0.0$ | $123.8 \pm 1.3$ | 2 | W | $145.4 \pm 1.5$ | $141.2 \pm 1.2$ | | | | | | |
| | 6 | W | $140.5 \pm 0.7$ | $131.2 \pm 0.0$ | 3 | W | $144.5 \pm 2.0$ | $142.2 \pm 0.1$ | 1 | CB | $144.5 \pm 1.9$ | $140.2 \pm 1.7$ | -1.26 | (a) |
| | 10 | CB | $140.9 \pm 0.1$ | $136.5 \pm 0.0$ | 2 | CB | $144.5 \pm 1.9$ | $141.7 \pm 0.9$ | | | | | | |
| | | | | | 5 | CB | $145.4 \pm 1.5$ | $141.2 \pm 1.5$ | 2 | CB | $144.6 \pm 1.9$ | $140.7 \pm 1.7$ | -0.42 | (a) |
| | | | | | 8 | W | $145.4 \pm 1.5$ | $142.2 \pm 0.0$ | | | | | | |
| | 14 | CB | $140.8 \pm 0.0$ | $136.5 \pm 0.0$ | 2 | CB | $144.6 \pm 2.0$ | $141.2 \pm 1.1$ | | | | | | |
| | | | | | 7 | CB | $143.7 \pm 1.8$ | $139.7 \pm 1.6$ | 3 | CB | $143.8 \pm 2.0$ | $140.7 \pm 1.8$ | 0.42 | (c) |
| | | | | | 10 | W | $143.8 \pm 1.8$ | $141.2 \pm 1.6$ | 3 | CB | $143.8 \pm 1.9$ | $140.7 \pm 1.7$ | 1.68 | (c) |
| | | | | | | | | | 6 | CB | $143.8 \pm 2.0$ | $140.2 \pm 1.6$ | | (c) |
| | | | | | 12 | W | $143.0 \pm 1.5$ | $140.3 \pm 1.8$ | | | | | | |
| 7 | 4 | W | $137.3 \pm 1.0$ | $120.5 \pm 0.3$ | | | | | | | | | | |
| | 6 | W | $142.9 \pm 1.9$ | $128.0 \pm 0.6$ | | | | | | | | | | |
| | 8 | W | $142.7 \pm 1.9$ | $129.2 \pm 0.0$ | | | | | | | | | | |
| | 10 | W | $144.1 \pm 0.0$ | $135.0 \pm 1.7$ | | | | | | | | | | |
| | 12 | W | $143.7 \pm 0.8$ | $139.1 \pm 1.0$ | | | | | | | | | | |
| 8 | 4 | W | $135.1 \pm 0.0$ | $116.9 \pm 0.2$ | 2 | W | $147.4 \pm 0.0$ | $137.4 \pm 0.0$ | | | | | | |
| | 6 | W | $147.7 \pm 0.2$ | $121.9 \pm 1.4$ | 3 | W | $148.2 \pm 0.0$ | $143.5 \pm 0.1$ | 1 | W | $148.2 \pm 0.1$ | $142.5 \pm 0.9$ | -1.26 | (a) |
| | 7 | W | $147.8 \pm 0.0$ | $124.5 \pm 0.9$ | 6 | W | $148.6 \pm 0.1$ | $127.3 \pm 0.1$ | 1 | W | $148.3 \pm 0.0$ | $127.3 \pm 0.2$ | 0 | (e) |
| | | | | | | | | | 2 | W | $148.3 \pm 0.0$ | $129.6 \pm 1.2$ | | |
| | 8 | W | $147.9 \pm 0.0$ | $126.5 \pm 0.1$ | 2 | W | $148.2 \pm 0.0$ | $143.8 \pm 0.2$ | | | | | | |
| | | | | | 4 | W | $148.2 \pm 0.0$ | $137.2 \pm 0.6$ | 2 | W | $148.1 \pm 0.1$ | $144.3 \pm 0.8$ | -0.84 | (a) |
| | | | | | 6 | W | $148.2 \pm 0.0$ | $129.9 \pm 1.6$ | 1 | W | $148.3 \pm 0.0$ | $131.8 \pm 1.0$ | 0 | (e) |
| | 10 | W | $147.9 \pm 0.1$ | $131.2 \pm 0.2$ | 2 | W | $148.3 \pm 0.0$ | $144.3 \pm 0.7$ | | | | | | |
| | | | | | 5 | W | $148.2 \pm 0.0$ | $137.8 \pm 0.0$ | 2 | W | $148.2 \pm 0.0$ | $139.7 \pm 1.5$ | -0.42 | (a) |
| | 12 | W | $147.9 \pm 0.1$ | $132.6 \pm 1.3$ | 10 | W | $148.2 \pm 0.1$ | $137.9 \pm 0.0$ | 2 | W | $148.3 \pm 0.1$ | $138.9 \pm 2.0$ | 1.68 | (c) |
| | 16 | CB | $147.9 \pm 0.0$ | $137.7 \pm 0.0$ | 4 | CB | $148.2 \pm 0.0$ | $143.8 \pm 0.1$ | 2 | CB | $148.2 \pm 0.0$ | $143.7 \pm 0.1$ | -0.84 | (a) |
| | | | | | 8 | W | $148.2 \pm 0.0$ | $143.9 \pm 0.1$ | 2 | CB | $148.1 \pm 0.1$ | $143.9 \pm 0.1$ | 0.84 | (c) |
| | | | | | | | | | 5 | CB | $148.2 \pm 0.0$ | $143.9 \pm 0.1$ | | (c) |
| | | | | | 12 | W | $148.2 \pm 0.0$ | $143.8 \pm 0.1$ | 2 | W | $148.2 \pm 0.0$ | $143.7 \pm 0.1$ | 2.52 | (b) |
| | | | | | | | | | 5 | CB | $148.4 \pm 0.1$ | $143.7 \pm 0.2$ | | (c) |
| | | | | | | | | | 9 | CB | $148.3 \pm 0.1$ | $144.0 \pm 0.1$ | | (c) |
| | | | | | 14 | W | $148.2 \pm 0.0$ | $143.9 \pm 0.0$ | | | | | | |
| | | | | | 15 | W | $148.5 \pm 0.1$ | $140.9 \pm 2.3$ | 2 | W | $148.3 \pm 0.1$ | $144.0 \pm 0.0$ | 3.79 | (b) |
| | 22 | CB | $147.9 \pm 0.0$ | $137.7 \pm 0.0$ | 4 | CB | $148.2 \pm 0.0$ | $143.8 \pm 0.1$ | 2 | CB | $148.3 \pm 0.0$ | $143.9 \pm 0.1$ | -0.84 | (a) |
| | | | | | 10 | W | $148.2 \pm 0.0$ | $143.8 \pm 0.2$ | 3 | CB | $148.2 \pm 0.0$ | $143.8 \pm 0.2$ | 1.68 | (c) |
| | | | | | | | | | 7 | CB | $148.2 \pm 0.1$ | $143.8 \pm 0.1$ | | (c) |
| | | | | | 18 | W | $148.5 \pm 0.1$ | $143.9 \pm 0.0$ | 3 | W | $148.2 \pm 0.0$ | $143.9 \pm 0.1$ | 5.05 | (b) |
| | | | | | | | | | 7 | CB | $148.2 \pm 0.0$ | $143.8 \pm 0.2$ | | (c) |
| | | | | | | | | | 15 | CB | $148.2 \pm 0.0$ | $143.8 \pm 0.2$ | | (c) |
| | | | | | 19 | W | $148.2 \pm 0.0$ | $143.9 \pm 0.1$ | 2 | W | $148.2 \pm 0.1$ | $143.8 \pm 0.1$ | 5.47 | (b) |
| | | | | | 21 | W | $148.4 \pm 0.1$ | $145.0 \pm 1.7$ | 2 | W | $148.3 \pm 0.0$ | $144.9 \pm 1.6$ | 6.31 | (b) |
| | 30 | CB | $147.9 \pm 0.0$ | $137.7 \pm 0.0$ | | | | | | | | | | |
| 9 | 4 | W | $132.6 \pm 0.0$ | $114.7 \pm 1.8$ | | | | | | | | | | |
| | 6 | W | $146.0 \pm 1.2$ | $116.6 \pm 1.9$ | | | | | | | | | | |
| | 8 | W | $146.5 \pm 0.0$ | $119.0 \pm 0.4$ | | | | | | | | | | |
| | 10 | W | $146.5 \pm 0.0$ | $124.4 \pm 0.6$ | | | | | | | | | | |
| | 12 | W | $145.9 \pm 1.1$ | $128.8 \pm 0.1$ | | | | | | | | | | |

| a | h | TS | $\theta_1^{\mathrm{CB,sim}}(^\circ)$ | $\theta_1^{\mathrm{W,sim}}(^\circ)$ | $h_2$ | TS | $\theta_2^{\mathrm{CB,sim}}(^\circ)$ | $\theta_2^{\mathrm{W,sim}}(^\circ)$ | $h_3$ | TS | $\theta_3^{\mathrm{CB,sim}}(^\circ)$ | $\theta_3^{\mathrm{W,sim}}(^\circ)$ | $h_3^*$ | Condition |
|---|---|---|---|---|---|---|---|---|---|---|---|---|---|---|
| 10 | 4 | W | $130.0 \pm 0.0$ | $115.4 \pm 1.3$ | 2 | W | $144.0 \pm 0.0$ | $128.6 \pm 0.0$ | | | | | | |
| | 6 | W | $148.6 \pm 1.7$ | $113.5 \pm 2.5$ | 3 | W | $150.9 \pm 0.0$ | $138.2 \pm 1.4$ | 1 | W | $150.9 \pm 0.1$ | $136.4 \pm 2.1$ | -1.26 | **(a)** |
| | | | | | 4 | W | $150.5 \pm 1.0$ | $126.0 \pm 0.9$ | 2 | W | $150.0 \pm 1.7$ | $138.2 \pm 1.5$ | -0.84 | **(a)** |
| | | | | | 5 | W | $151.6 \pm 0.1$ | $127.1 \pm 0.3$ | 3 | W | $151.4 \pm 0.1$ | $139.4 \pm 0.1$ | -0.42 | **(a)** |
| | 7 | W | $147.9 \pm 2.1$ | $111.5 \pm 2.4$ | 6 | W | $151.5 \pm 0.0$ | $126.9 \pm 0.1$ | 2 | W | $151.4 \pm 0.0$ | $126.1 \pm 0.8$ | 0 | **(e)** |
| | | | | | | | | | 3 | W | $151.4 \pm 0.0$ | $126.8 \pm 0.2$ | | |
| | | | | | | | | | 4 | W | $151.4 \pm 0.0$ | $140.1 \pm 0.2$ | | |
| | 8 | W | $147.9 \pm 2.1$ | $115.1 \pm 1.5$ | 2 | W | $151.0 \pm 0.1$ | $139.5 \pm 0.1$ | | | | | | |
| | | | | | 4 | W | $150.4 \pm 0.9$ | $126.3 \pm 1.7$ | 2 | W | $150.3 \pm 1.1$ | $140.1 \pm 0.1$ | -0.84 | **(a)** |
| | | | | | 5 | W | $150.4 \pm 1.0$ | $125.5 \pm 1.6$ | 2 | W | $150.4 \pm 1.1$ | $126.5 \pm 0.9$ | -0.42 | **(a)** |
| | | | | | 6 | W | $150.9 \pm 0.1$ | $126.1 \pm 0.8$ | 1 | W | $151.1 \pm 0.1$ | $126.4 \pm 0.9$ | 0 | **(e)** |
| | | | | | | | | | 2 | W | $150.5 \pm 0.9$ | $126.6 \pm 0.3$ | | |
| | | | | | 7 | W | $151.6 \pm 0.1$ | $127.0 \pm 0.2$ | 2 | W | $151.4 \pm 0.0$ | $126.2 \pm 0.8$ | 0.42 | **(c)** |
| | 10 | W | $148.5 \pm 1.7$ | $116.9 \pm 1.6$ | 2 | W | $150.4 \pm 1.0$ | $142.2 \pm 2.3$ | | | | | | |
| | | | | | 5 | W | $151.1 \pm 0.1$ | $127.1 \pm 0.6$ | 2 | W | $150.5 \pm 1.1$ | $126.1 \pm 1.8$ | -0.42 | **(a)** |
| | | | | | 6 | W | $150.6 \pm 0.9$ | $126.3 \pm 0.9$ | 1 | W | $151.0 \pm 0.1$ | $126.2 \pm 0.9$ | 0 | **(e)** |
| | | | | | | | | | 2 | W | $150.7 \pm 0.7$ | $127.7 \pm 0.8$ | | |
| | | | | | 8 | W | $151.0 \pm 0.2$ | $126.0 \pm 1.5$ | | | | | | |
| | 12 | W | $148.2 \pm 1.9$ | $119.5 \pm 0.4$ | 6 | W | $151.0 \pm 0.2$ | $128.4 \pm 1.7$ | 1 | W | $150.9 \pm 0.1$ | $129.5 \pm 2.1$ | 0 | **(e)** |
| | | | | | | | | | 2 | W | $150.7 \pm 0.6$ | $132.9 \pm 0.7$ | | |
| | 14 | W | $148.1 \pm 1.5$ | $123.7 \pm 1.9$ | 2 | W | $151.0 \pm 0.2$ | $145.8 \pm 0.2$ | | | | | | |
| | | | | | 7 | W | $150.3 \pm 0.9$ | $132.8 \pm 1.0$ | 4 | W | $149.4 \pm 1.9$ | $141.8 \pm 1.7$ | 0.42 | **(c)** |
| | | | | | 10 | W | $150.9 \pm 0.3$ | $128.5 \pm 1.0$ | 3 | W | $150.2 \pm 1.5$ | $133.1 \pm 0.5$ | 1.68 | **(c)** |
| | | | | | | | | | 7 | CB | $149.3 \pm 1.7$ | $145.4 \pm 0.3$ | | **(c)** |
| | | | | | 12 | W | $151.1 \pm 0.2$ | $129.3 \pm 2.0$ | | | | | | |
| | 16 | W | $147.8 \pm 1.8$ | $127.8 \pm 1.2$ | 15 | W | $151.5 \pm 0.0$ | $129.6 \pm 1.5$ | 2 | W | $151.4 \pm 0.1$ | $132.5 \pm 2.3$ | 3.79 | **(b)** |
| | 18 | W | $147.9 \pm 1.8$ | $132.1 \pm 0.0$ | 6 | W | $150.6 \pm 1.1$ | $145.0 \pm 0.3$ | 3 | CB | $150.4 \pm 1.0$ | $145.8 \pm 0.1$ | 0 | **(e)** |
| | | | | | 14 | W | $149.9 \pm 1.6$ | $139.6 \pm 0.0$ | 2 | W | $150.5 \pm 1.0$ | $145.7 \pm 0.1$ | 3.36 | **(b)** |
| | | | | | | | | | 3 | W | $150.5 \pm 1.0$ | $145.9 \pm 0.2$ | | **(b)** |
| | | | | | | | | | 7 | CB | $150.9 \pm 0.3$ | $145.8 \pm 0.1$ | | **(c)** |
| | | | | | | | | | 11 | CB | $149.8 \pm 1.2$ | $145.8 \pm 0.0$ | | **(c)** |
| | | | | | 17 | W | $151.6 \pm 0.0$ | $132.7 \pm 0.0$ | | | | | | |
| | 22 | W | $146.9 \pm 1.4$ | $139.7 \pm 1.0$ | 2 | CB | $150.5 \pm 0.9$ | $145.8 \pm 0.1$ | | | | | | |
| | | | | | 14 | W | $150.0 \pm 1.0$ | $145.7 \pm 0.1$ | 3 | W | $150.0 \pm 1.3$ | $145.7 \pm 0.2$ | 3.36 | **(b)** |
| | | | | | | | | | 7 | CB | $151.0 \pm 0.1$ | $146.2 \pm 1.1$ | | **(c)** |
| | | | | | | | | | 11 | CB | $150.0 \pm 1.3$ | $145.8 \pm 0.0$ | | **(c)** |
| | | | | | 18 | W | $150.9 \pm 0.2$ | $142.0 \pm 1.7$ | 3 | W | $150.8 \pm 0.5$ | $145.9 \pm 0.2$ | 5.05 | **(b)** |
| | | | | | | | | | 7 | W | $150.4 \pm 1.1$ | $145.9 \pm 0.1$ | | **(c)** |
| | | | | | | | | | 11 | CB | $150.9 \pm 0.1$ | $145.8 \pm 0.1$ | | **(c)** |
| | | | | | | | | | 15 | CB | $150.3 \pm 1.1$ | $145.8 \pm 0.3$ | | **(c)** |
| | | | | | 21 | W | $151.5 \pm 0.0$ | $133.0 \pm 0.4$ | 4 | W | $151.4 \pm 0.1$ | $146.2 \pm 0.2$ | 6.31 | **(b)** |
| | | | | | | | | | 5 | W | $151.6 \pm 0.1$ | $146.1 \pm 0.1$ | | **(b)** |

Figure S2: The table shows simulated points which are presented in the scatter plot, Fig(7). $\theta_i^{\mathrm{CB,sim}}$ and $\theta_i^{\mathrm{W,sim}}$ are the average of contact angle over 5 runs, initiating in the wetting state $CB^0$ and $W^0$ respectively. Geometric parameters (a, h, $h_2$, $h_3$) are in units of $\mu$m. The column "TS" shows the the theoretical wetting state predicted by the model for each geometry (indicated in the column "condition"). All the simulations have $w = 10$ $\mu$m, $w_2 = 2$ $\mu$m and $w_3 = 1$ $\mu$m.

# Notes and References


(1) Fernandes, H. C. M.; Vainstein, M. H.; Brito, C. Modeling of Droplet Evaporation on Superhydrophobic Surfaces. *Langmuir* **2015**, *31*, 7652–7659.

(2) de Oliveira, L. R.; Lopes, D. M.; Ramos, S. M. M.; Mombach, J. C. M. Two-dimensional modeling of the superhydrophobic behavior of a liquid droplet sliding down a ramp of pillars. *Soft Matter* **2011**, *7*, 3763–3765.

(3) Lopes, D. M.; de Oliveira, L. R.; Ramos, S. M. M.; Mombach, J. C. M. Cassie-Baxter to Wenzel state wetting transition: a 2D numerical simulation. *RSC Adv.* **2013**, *3*, 24530–24534.

(4) Mortazavi, V.; D'Souza, R. M.; Nosonovsky, M. Study of contact angle hysteresis using the cellular Potts model. *Phys. Chem. Chem. Phys.* **2013**, *15*, 2749–2756.

(5) The interface sites are defined as the ones which have at least one neighbor in a different state than its own, among the 18 first and second closest neighbors. This smaller neighborhood (compared to the Moore neighborhood) is used so that it is possible to obtain spherical droplets, despite the underlying lattice symmetries.

(6) Graner, F.; Glazier, J. A. Simulation of biological cell sorting using a two-dimensional extended Potts model. *Phys. Rev. Lett.* **1992**, *69*, 2013–2017.

(7) Tsai, P.; Lammertink, R.; Wessling, M.; Lohse, D. Evaporation-triggered wetting transition for water droplets upon hydrophobic microstructures. *Phys. Rev. Lett.* **2010**, *104*, 116102.
